# Supplementary material for: Blades: A Unified Benchmark Suite for Byzantine Attacks and Defenses in Federated Learning
Source: arXiv:2206.05359 source file (2023-11-10)
Supplement: Supplementary file 2 [file appendix.tex]

\begin{comment}
\subsection{Implementation Details}
\subsubsection{Important Callbacks of \ours}
\begin{table*}[ht]
\begin{center}
\begin{tabular}{c|l|l}
     Module & Callback Name & Example Use Case  \\
     \hline
     Server & \code{aggregate()}  & Adaptive/robust aggregation\\
     Server & \code{global\_update()}  & Server-side optimization\\
     \hline
     Client Manager & \code{omniscient\_callback()}  & Full knowledge attacks\\
     Client Manager & \code{select\_participants()}  & Client selection\\
     \hline
     Client & \code{on\_batch\_begin()}  &  Attacking single batch of training data (e.g., Label Flipping attack)\\
     Client & \code{on\_backward\_end()}  & Gradient manipulation (e.g., Sign Flipping attack)\\
     Client & \code{train()}  & Local SGD/in-depth attack customization\\
\hline

\end{tabular}
\vspace{0.1cm}
\caption{Some Callbacks. \ours provides APIs to integrate new plugins for various designs. We omit input arguments for brevity here.}
\label{callbacks}
\end{center}
\end{table*}
\end{comment}

\subsection{Additional Experimental Results}

Figure~\ref{atk_local_20} shows the results of aggregation rules using 20 steps of local updates, i.e., $E_l=20$. The observed robustness patterns are partially consistent with those described Section~\ref{sec_agg} where we set $E_l=1$, i.e., traditional GARs (i.e., \median~\cite{yin2018byzantine}, \tm~\cite{yin2018byzantine}, and \gm~\cite{pillutla2022robust}) still exhibit greater vulnerabilities to attacks compared to EGARs. However, Figure~\ref{atk_local_20} reveals a greater diversity in the robustness of aggregation rules when utilizing the Fashion MNIST dataset. Particularly, the SignFlipping attack causes a significant accuracy drop to most defenses when down to $15\%$ of the clients are malicious. Notably, \clippedclustering exhibits effective defense against all examined attacks without substantial degradation in performance, whereas other aggregation rules manifest vulnerabilities to specific attack types.

\begin{figure*}[ht]
	\begin{subfigure}[b]{\linewidth}
		\centering
		\includegraphics[width=\linewidth]{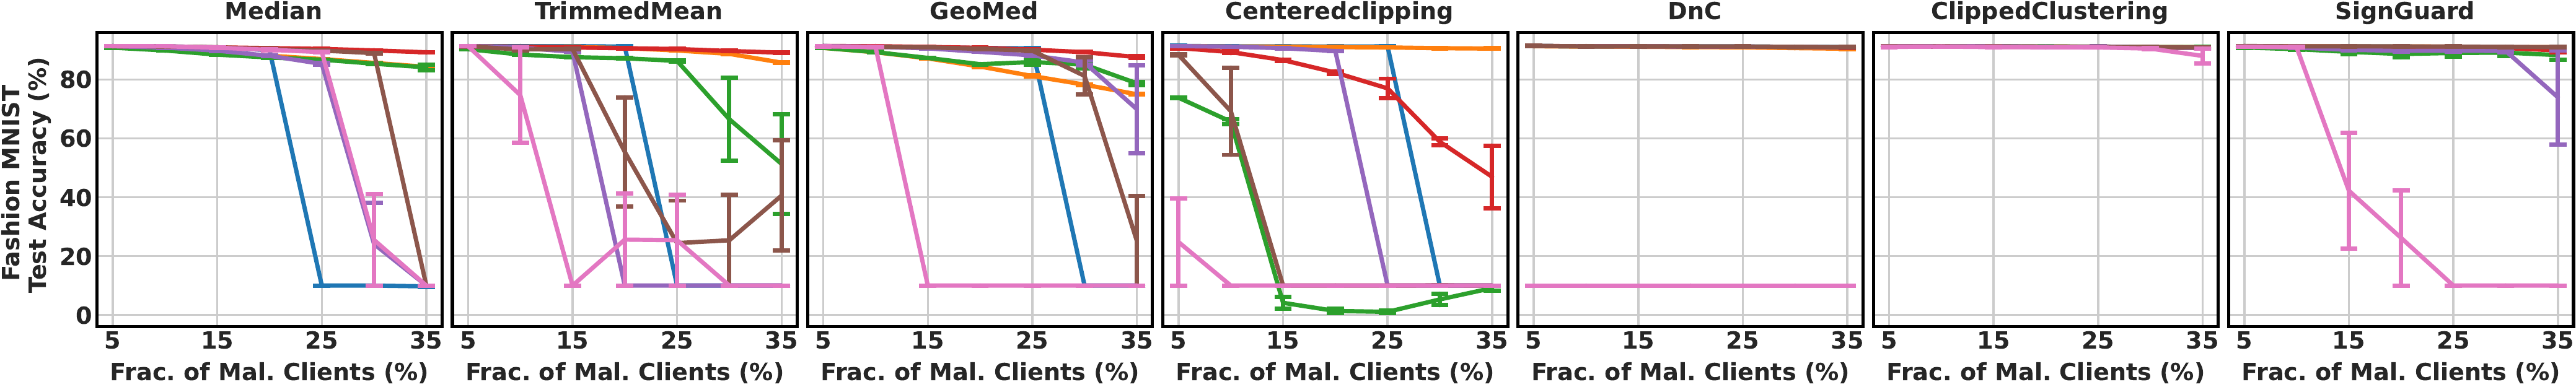}
	\end{subfigure}
	\begin{subfigure}[b]{\linewidth}
		\centering
		\includegraphics[width=\linewidth]{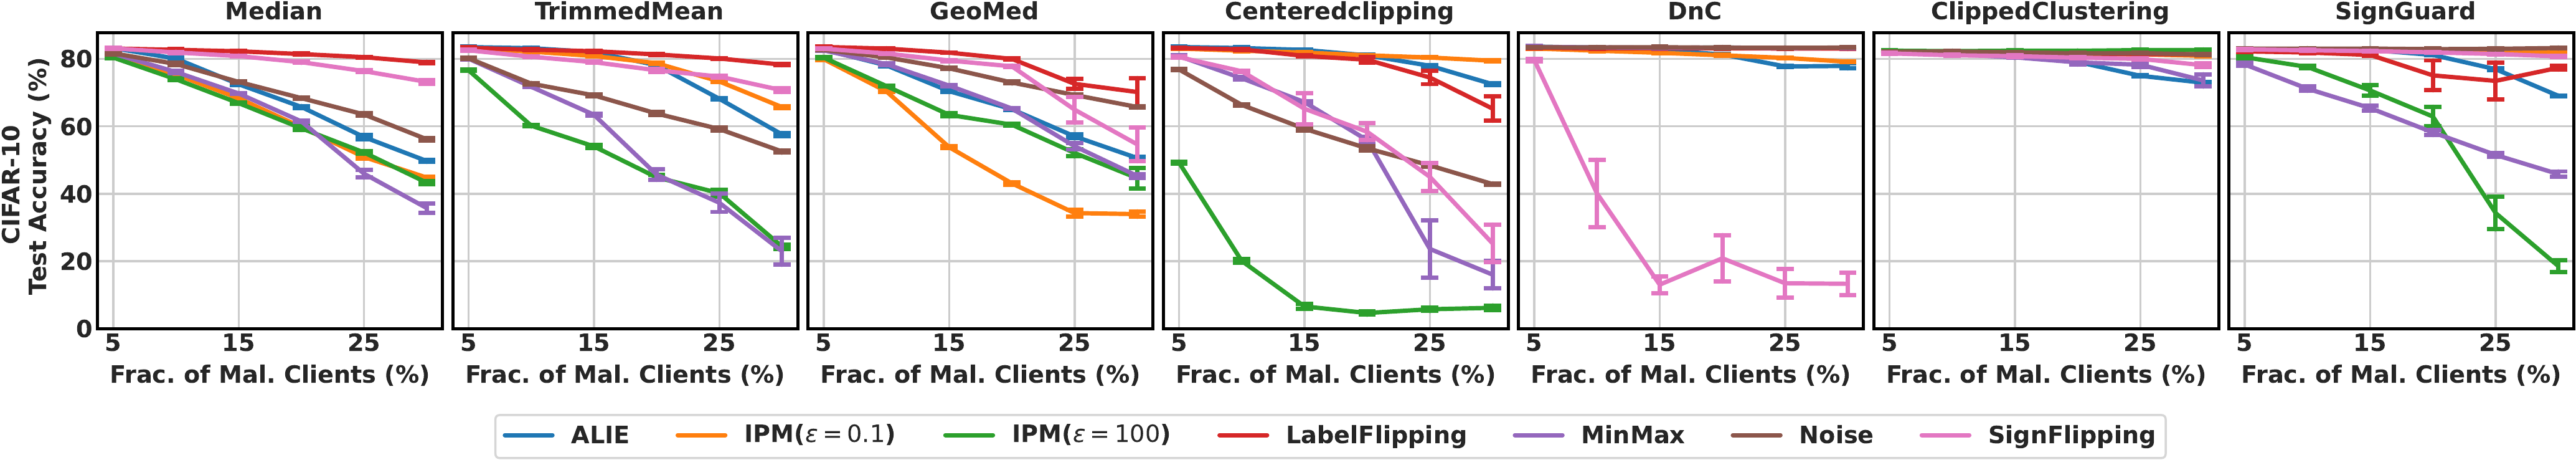}
	\end{subfigure}
% 	\vspace*{-0.5cm}
	\caption{Comparing state-of-the-art aggregation rules under various attacks on Fashion MNIST and CIFAR10 datasets with IID partition. Unlike the settings described in Section~\ref{sec_agg}, we utilize 20 steps for local updates (i.e., $E_l=20$). Similarly, traditional GARs (i.e., \median~\cite{yin2018byzantine}, \tm~\cite{yin2018byzantine}, and \gm~\cite{pillutla2022robust}) still exhibit greater vulnerabilities to attacks, whereas advanced EGARs display greater resilience against the majority of attacks. Notably, \clippedclustering exhibits effective defense against all examined attacks without substantial degradation in performance, whereas other aggregation rules manifest vulnerabilities to specific attack types.}
	\label{atk_local_20}
\end{figure*}
